# Supplementary material for: Differentially Private AUC Computation in Vertical Federated Learning
Source: arXiv:2205.12412 source file (2022-05-24)
Supplement: Supplementary file 1 [file leakage_from_prediction_score.tex]

\section{Potential Label Leakage from the Prediction Scores}
\label{sec:label_leakage_from_prediction_scores}

% \input{tables/top_k_analysis_production_data}

% \begin{figure*}[ht!]% \vspace{-0.1in}
%   \centering
%     \includegraphics[width=1.0\linewidth]{figures/production_negative_positive_density.pdf}
%   \caption{Density of positive and negative instances' prediction scores in production data.}
%  \label{fig:production_negative_positive_density}
%  \end{figure*}
